# Supplementary material for: Hierarchy Denoising Recursive Autoencoders for 3D Scene Layout Prediction
Source: arXiv:1903.03757 source file (2019-04-10)
Supplement: Supplementary file 1 [file appendix.tex]

\appendix

\section{Spatial Relationship Descriptor}
\label{sec:spatial_descriptor}

The spatial relationship descriptor $D_s$ captures the spatial relationship between the bounding boxes of two object nodes.
Following \citet{liu2014creating}, we define $D_s(n_i,n_j)$ between two nodes $n_i$ and $n_j$ as a 7-dimensional vector:

\begin{align*}
D_s(n_i,n_j) =[ &n_i.z_{min}-n_j.z_{min},\\
&n_i.z_{min}-n_j.z_{max},\\
&n_i.z_{max}-n_j.z_{min},\\
&\lVert n_i\text{.box.center} - n_j\text{.box.center} \rVert,\\
&\textbf{Dist}(n_i\text{.box}, n_j\text{.box}),\\
&\textbf{Vol}(n_i\text{.box}\cap n_j\text{.box})/\textbf{Vol}(n_i\text{.box}),\\
&\textbf{Vol}(n_i\text{.box}\cap n_j\text{.box})/\textbf{Vol}(n_j\text{.box})]
\end{align*}

Intuitively, the first three components describe the relative height of the two objects and capture the vertical relationship between them. The fourth component is the Euclidean distance between the centroids of $n_i$ and $n_j$. The fifth is the distance between the two bounding boxes defined as the closest distance between all pairs of points on those two bounding boxes. The last two components represent the amount of overlap between the two regions.
